# Supplementary material for: An Empirical Investigation of Randomized Defenses against Adversarial Attacks
Source: arXiv:1909.05580 source file (2019-09-12)
Supplement: Supplementary file 1 [file robu-appendix.tex]

\begin{figure}[h!]
    \centering
    \begin{tikzpicture}[baseline]
        %%% FIRST LEFT %%%
        \begin{axis}[
            width=0.5\columnwidth,
            height=0.20\textheight,
            xmode=log,
            log basis x={2},
            log ticks with fixed point,% Turn 2^1.00, 2^2.00, ... to 2, 4, ...
            ymin=0,
            ymax=0.7,
            y tick label style={
                /pgf/number format/.cd,
                    fixed,
                    precision=1,
                /tikz/.cd
            },
        ]
            \addplot+[mark options={scale=0.5}]table [x=n,y=0.5-robustness] {data/robustness/robustness_of_pwg_on_vgg19_fgsm_99settings.csv};
            \addplot+[mark options={scale=0.5}]table [x=n,y=0.8-robustness] {data/robustness/robustness_of_pwg_on_vgg19_fgsm_99settings.csv};
            \addplot+[mark options={scale=0.5}]table [x=n,y=0.95-robustness] {data/robustness/robustness_of_pwg_on_vgg19_fgsm_99settings.csv};
            \addplot+[mark options={scale=0.5}]table [x=n,y=0.99-robustness] {data/robustness/robustness_of_pwg_on_vgg19_fgsm_99settings.csv};
            \addplot+[mark options={scale=0.5}]table [x=n,y=1-robustness] {data/robustness/robustness_of_pwg_on_vgg19_fgsm_99settings.csv};
        \end{axis}
    \end{tikzpicture}
    %%% FIRST RIGHT %%%
    \begin{tikzpicture}[baseline]
        \begin{axis}[
            width=0.5\columnwidth,
            height=0.20\textheight,
            xmode=log,
            log basis x={2},
            log ticks with fixed point,% Turn 2^1.00, 2^2.00, ... to 2, 4, ...
            ymin=0,
            ymax=0.7,
            yticklabel pos=upper,
            y tick label style={
                /pgf/number format/.cd,
                    fixed,
                    precision=1,
                /tikz/.cd
            },
            legend style={font=\scriptsize},
            legend entries={
                $\robustness{0.50}{n}$,
                $\robustness{0.80}{n}$,
                $\robustness{0.95}{n}$,
                $\robustness{0.99}{n}$,
                $\robustness{1.00}{n}$
            },
        ]
            \addplot+[mark options={scale=0.5}]table [x=n,y=0.5-robustness] {data/robustness/robustness_of_pwg_on_vgg19_fgsm_98settings.csv};
            \addplot+[mark options={scale=0.5}]table [x=n,y=0.8-robustness] {data/robustness/robustness_of_pwg_on_vgg19_fgsm_98settings.csv};
            \addplot+[mark options={scale=0.5}]table [x=n,y=0.95-robustness] {data/robustness/robustness_of_pwg_on_vgg19_fgsm_98settings.csv};
            \addplot+[mark options={scale=0.5}]table [x=n,y=0.99-robustness] {data/robustness/robustness_of_pwg_on_vgg19_fgsm_98settings.csv};
            \addplot+[mark options={scale=0.5}]table [x=n,y=1-robustness] {data/robustness/robustness_of_pwg_on_vgg19_fgsm_98settings.csv};
        \end{axis}
    \end{tikzpicture}
    \begin{tikzpicture}[baseline]
        %%% SECOND LEFT %%%
        \begin{axis}[
            width=0.5\columnwidth,
            height=0.20\textheight,
            xmode=log,
            log basis x={2},
            log ticks with fixed point,% Turn 2^1.00, 2^2.00, ... to 2, 4, ...
            xlabel={$n$},
            ymin=0.0,
            ymax=0.5,
            y tick label style={
                /pgf/number format/.cd,
                    fixed,
                    precision=1,
                /tikz/.cd
            },
        ]
            \addplot+[mark options={scale=0.5}]table [x=n,y=0.5-robustness] {data/robustness/robustness_of_pwg_on_vgg19_sma_99settings.csv};
            \addplot+[mark options={scale=0.5}]table [x=n,y=0.8-robustness] {data/robustness/robustness_of_pwg_on_vgg19_sma_99settings.csv};
            \addplot+[mark options={scale=0.5}]table [x=n,y=0.95-robustness] {data/robustness/robustness_of_pwg_on_vgg19_sma_99settings.csv};
            \addplot+[mark options={scale=0.5}]table [x=n,y=0.99-robustness] {data/robustness/robustness_of_pwg_on_vgg19_sma_99settings.csv};
            \addplot+[mark options={scale=0.5}]table [x=n,y=1-robustness] {data/robustness/robustness_of_pwg_on_vgg19_sma_99settings.csv};
        \end{axis}
    \end{tikzpicture}
    %%% SECOND RIGHT %%%
    \begin{tikzpicture}[baseline]
        \begin{axis}[
            width=0.5\columnwidth,
            height=0.20\textheight,
            xmode=log,
            log basis x={2},
            log ticks with fixed point,% Turn 2^1.00, 2^2.00, ... to 2, 4, ...
            xlabel={$n$},
            ymin=0,
            ymax=0.5,
            yticklabel pos=upper,
            y tick label style={
                /pgf/number format/.cd,
                    fixed,
                    precision=1,
                /tikz/.cd
            },
        ]
            \addplot+[mark options={scale=0.5}]table [x=n,y=0.5-robustness] {data/robustness/robustness_of_pwg_on_vgg19_sma_98settings.csv};
            \addplot+[mark options={scale=0.5}]table [x=n,y=0.8-robustness] {data/robustness/robustness_of_pwg_on_vgg19_sma_98settings.csv};
            \addplot+[mark options={scale=0.5}]table [x=n,y=0.95-robustness] {data/robustness/robustness_of_pwg_on_vgg19_sma_98settings.csv};
            \addplot+[mark options={scale=0.5}]table [x=n,y=0.99-robustness] {data/robustness/robustness_of_pwg_on_vgg19_sma_98settings.csv};
            \addplot+[mark options={scale=0.5}]table [x=n,y=1-robustness] {data/robustness/robustness_of_pwg_on_vgg19_sma_98settings.csv};
        \end{axis}
    \end{tikzpicture}
    \caption{
        Estimated $\robuvar(\text{\dmnamesing}, \robulevel, \ninstalls)$ using $(\reldev, \esbsize) = (0.05, 7)$ (left graphs) and $(\reldev, \esbsize) = (0.11, 63)$ (right graphs), evaluated against the AE generation methods \AEMfgsm\ (top row) and \AEMsma\ (bottom row).
    }
    \label{fig:robu-appendix}
\end{figure}
